# Supplementary material for: Linear Absorption Spectrum of the Spin-Boson Model Studied by Extended Hierarchical Equations of Motion
Source: arXiv:2302.01908 source file (2023-02-03)
Supplement: Supplementary file 1 [file supplementary.pdf]

# Supplementary Materials for "Linear Absorption Spectra of the Spin-Boson Model Studied by Extended Hierarchical Equations of Motion"

Qianlong Wang[1] and Jianlan Wu[1,*]

[1]*Physics Department, Zhejiang University, Hangzhou, Zhejiang, 310027, China*

[*]Electronic address: jianlanwu@zju.edu.cn

In this supporting material, we present the definition of linear response function, the derivation of extended HEOM and several complex initial states that can be obtained from the system-bath factorized state. As a demonstration, we show two typical initial states: the local equilibrium state and the excited equilibrium state. With the assistance of complete dynamic set, the resemblance between quantum operations and HEOM matrices is introduced. In order to calculate the linear response function, the extended HEOM applied to a excited equilibrium initial state is required.

## I. LINEAR RESPONSE FUNCTION

With the consideration of an external electromagnetic field, the total Hamiltonian experienced by the sample is written as

$$H_{\rm tot}(t) = H_0 + H_{\rm ext}(t), \tag{1}$$

where $H_0 = H_{\rm S} + H_{\rm B} + H_{\rm SB}$ is the Hamiltonian of spin-boson model and $H_1(t)$ is the time-dependent external Hamiltonian. The external Hamiltonian between the spin system and the external field is assumed as

$$H_{\rm ext}(t) = -\hat{\mu} \cdot \vec{E}(t), \tag{2}$$

where $\hat{\mu}$ is the dipole moment vector operator. $\vec{E}(t)$ is the external electric field, which set as along the $z$ axis, $\vec{E}(t) = E(t)\vec{e}_z$. In this paper, $\hat{\mu}$ only have the non-diagonal elements to realize the transition between the ground state and excited state. The longitudinal component of $\hat{\mu}$ is $\hat{\mu} = \mu_z\sigma_z$. $\mu_z$ is the non-diagonal element of the dipole moment operator. Thus the external Hamiltonian can be re-expressed as $H_1(t) = -\mu_z\sigma_z E(t)$. The time-dependent electric field can be seen as a periodic perturbation, which will lead to an oscillation between the ground state $|g\rangle$ and excited state $|e\rangle$. This corresponds to the process of energy resonance absorption and it can be reflected in the linear absorption spectra.

In the interaction picture, the time evolution operator $U_0(t, t_0)$ is ($\hbar = 1$)

$$U_0(t, t_0) = U_0(t)U_0^\dagger(t_0) = e^{-iH_0(t-t_0)}, \tag{3}$$

here $U_0(t) = e^{-iH_0t}$ and $U_0(t_0) = e^{-iH_0t_0}$ are the operator related to the unpertubated Hamiltonian $H_0$. So the perturbed term in the interaction picture can be expressed as

$$H_1^I(t) = U_0(t_0)U_0^\dagger(t)H_1(t)U_0(t)U_0^\dagger(t_0) = -\mu_z\sigma_z(t)E(t). \tag{4}$$

To calculate the expectation of observable quantity, it's necessary to introduce the density operator. The time-dependent density operator $\rho^I(t)$ in the interaction picture can be expanded in powers of the external field, i.e.,

$$\rho^I(t) = \rho(t_0) + \rho_1^I(t) + \rho_2^I(t) + \cdots, \tag{5}$$

where $\rho_n^I(t)$ denotes the $n$th order contribution in the external field. In the initial time $t_0 = -\infty$, the zeroth order contribution $\rho(t_0) = \rho(-\infty)$ is the total density matrix operator in equilibrium state, which commutes with $H_0$ and $U_0(t)$, $[\rho(t_0), H_0] = [\rho(t_0), U_0(t)] = 0$.

Additionally, the density matrix operator $\rho^I(t)$ obeys the quantum Liouville equation

$$\frac{d}{dt}\rho^I(t) \ = -i[H_1^I(t), \rho^I(t)]. \tag{6}$$

Now let's only keep the zeroth order contribution $\rho^I(t) \approx \rho(t_0)$, then we integrate Eq. (6) from the initial time, giving

$$\begin{aligned}\rho^I(t) \ &= \ \rho(t_0) - i\int_{t_0}^{t}[H_1^I(\tau), \rho^I(\tau)]\, d\tau, \\ &\approx \ \rho(t_0) + i\mu_z\int_{t_0}^{t}[\sigma_z(\tau), \rho(t_0)]E(\tau)\, d\tau.\end{aligned} \tag{7}$$

In the interaction picture, the dipole moment operator is written as $\hat{\mu}(t) = U_0(t_0)U_0^\dagger(t)\hat{\mu}U_0(t)U_0^\dagger(t_0)$. Then in an optical measurement, the observable dipole moment operator at time $t$ can be expressed as

$$\begin{aligned}\langle\hat{\mu}(t)\rangle \ &= \ \mathrm{Tr}\{\hat{\mu}(t)\rho^I(t)\}, \\ &= \ \mathrm{Tr}\{\hat{\mu}(t)\rho(t_0)\} + i\mu_z^2\int_{t_0}^{t}\mathrm{Tr}\left\{\sigma_z(t)[\sigma_z(\tau), \rho(t_0)]\right\}E(\tau)d\tau.\end{aligned} \tag{8}$$

The first term can be simplified as the expectation of $\hat{\mu}(t)$ in equilibrium state

$$\begin{aligned}\mathrm{Tr}\{\hat{\mu}(t)\rho(t_0)\} \ &= \ \mathrm{Tr}\{\hat{\mu}(t)\rho(t_0)\}, \\ &= \ \mathrm{Tr}\{U_0(t_0)U_0^\dagger(t)\hat{\mu}U_0(t)U_0^\dagger(t_0)\rho(t_0)\}, \\ &= \ \mathrm{Tr}\{\hat{\mu}\rho(t_0)\}, \\ &= \ \langle\hat{\mu}(t_0)\rangle.\end{aligned} \tag{9}$$

Considering the time translation invariance, Eq. (8) can be further re-arranged into

$$\begin{aligned}\langle\hat{\mu}(t)\rangle - \langle\hat{\mu}(t_0)\rangle \ &= \ i\mu_z^2\int_{t_0}^{t}\mathrm{Tr}\{\sigma_z(t)[\sigma_z(\tau), \rho(t_0)]\}E(\tau)d\tau, \\ &= \ i\mu_z^2\int_{t_0}^{t}\mathrm{Tr}\{[\sigma_z(t), \sigma_z(\tau)]\rho(t_0)\}E(\tau)d\tau, \\ &= \ i\mu_z^2\int_{-\infty}^{\infty}\Theta(t-\tau)\mathrm{Tr}\{[\sigma_z(t-\tau), \sigma_z]\rho(-\infty)\}E(\tau)\, d\tau.\end{aligned} \tag{10}$$

here the Heaviside step function $\Theta(t-\tau)$ is used to extend the integral's upper limit to infinity.

A response function for a macroscopic system relates the change of dipole moment operator $\langle\hat{\mu}(t)\rangle$ to an external field $E(t)$. Thus the linear response function $\chi(t)$ is defined as

$$\langle\hat{\mu}(t)\rangle - \langle\hat{\mu}(t_0)\rangle = \int_{-\infty}^{\infty}\chi(t-\tau)E(\tau)\, d\tau. \tag{11}$$

Thus the Kubo formula is finally obtained by comparing this definition with Eq. (10),

$$\chi(t) \ = i\Theta(t)\mathrm{Tr}\{[\sigma_z(t), \sigma_z]\,\rho(-\infty)\}\mu_z^2, \tag{12}$$

where $\Theta(t)$ is the Heaviside function to keep the causality. The trace is taken over all the degrees of system and bath, $\mathrm{Tr} = \mathrm{Tr_S}\mathrm{Tr_B}$.

In order to calculate the linear response function with extended HEOM, we need to rewrite Eq. (12) in the formalism of extended HEOM. Firstly, with the invariance of the trace under cyclic permutations, Eq. (15) can be rewritten as

$$\begin{aligned}\chi(t) &= i\Theta(t)\mathrm{Tr}\{[\sigma_z(t),\sigma_z]\,\rho(-\infty)\}\mu_z^2,\\ &= i\Theta(t)\mathrm{Tr}\{\sigma_z(t)\,[\sigma_z,\rho(-\infty)]\}\mu_z^2. \end{aligned}\tag{13}$$

Furthermore, by using the Liouville superoperator $\mathcal{L}$, i.e. $\sigma_z(t)=\sigma_z e^{-i\mathcal{L}t}$ and $\mathcal{L}_z=[\sigma_z,\cdots]$, the linear response function is finally re-expressed as

$$\begin{aligned}\chi(t) &= i\Theta(t)\mathrm{Tr}\{\sigma_z(t)\,[\sigma_z,\rho(-\infty)]\}\mu_z^2,\\ &= i\Theta(t)\mathrm{Tr}\{\sigma_z e^{-i\mathcal{L}t}[\sigma_z,\rho(-\infty)])\}\mu_z^2,\\ &= i\Theta(t)\mathrm{Tr}_\mathrm{S}\{\sigma_z\mathrm{Tr}_\mathrm{B}\{e^{-i\mathcal{L}t}(\mathcal{L}_z\rho(-\infty))\}\}\mu_z^2. \end{aligned}\tag{14}$$

## II. DERIVATION OF THE EXTENDED HEOM FROM SYSTEM-BATH FACTORIZED INITIAL STATE

In the field of open quantum system, the extended HEOM is a non-perturbative kinetic method that can be applied to calculate the reduced density matrix of the system, $\rho_\mathrm{S}(t)=\mathrm{Tr}_\mathrm{B}\{\rho_\mathrm{tot}(t)\}$. We briefly review the derivation of the extended HEOM. To be consistent with the main text, we only consider the situation of an unbiased spin coupled with a bosonic bath. The derivation can be straightforwardly extended to an arbitrary quantum system.

The total Hamiltonian $H_\mathrm{tot}$ consists of three terms: the bare system Hamiltonian $H_\mathrm{S}$, the bare bath Hamiltonian $H_\mathrm{B}$, and their interaction $H_\mathrm{SB}$. $H_\mathrm{tot}$ is written as

$$H = H_\mathrm{S}+H_\mathrm{B}+H_\mathrm{SB}. \tag{15}$$

Here the system Hamiltonian of an unbiased spin reads $H_\mathrm{S}=\Delta\sigma_x$, with $\sigma_x$ the Pauli matrix and $\Delta$ the tunneling amplitude between two spin states. The Hamiltonian of the bosonic bath reads $H_\mathrm{B}=(1/2)\sum_j(p_j^2+\omega_j^2q_j^2)$, where $\omega_j$,$p_j$, and $q_j$ are the frequency, momentum and position of the $j$th harmonic oscillator. The system-bath interaction takes a bilinear form $H_\mathrm{SB}=\sigma_z\sum_j c_jq_j$, which subsequently defines the bath spectral density, $J(\omega)=(\pi/2)\sum_j(c_j^2/\omega_j)\delta(\omega-\omega_j)$, and the bath time correlation function,

$$C(t)=\frac{1}{\pi}\int_0^\infty J(\omega)[\coth(\frac{\beta\omega}{2})\cos(\omega t)-i\sin(\omega t)]\,d\omega. \tag{16}$$

To evaluate quantum dynamics of the spin system, we introduce the interaction picture of $H_0=H_\mathrm{S}+H_\mathrm{B}$. The time evolution of the total density matrix $\rho^I_\mathrm{tot}(t)$ is governed by the Liouville equation,

$$\partial_t\rho^I_\mathrm{tot}(t)=-\mathcal{L}_\mathrm{SB}(t)\rho^I_\mathrm{tot}(t), \tag{17}$$

where the superscript $I$ denotes the interaction picture, and the commutator $\mathcal{L}_\mathrm{SB}(t)=[H_\mathrm{SB},\cdots]$ is treated as a Liouville superoperator. The time-dependent system-bath interaction, $H_\mathrm{SB}(t)=\sigma_z(t)F(t)$, includes two parts, $\sigma_z(t)=\exp(iH_\mathrm{S}t)\sigma_z\exp(-iH_\mathrm{S}t)$ and $F(t)=\exp(iH_\mathrm{B}t)\sum_j c_jq_j\exp(-iH_\mathrm{B}t)$. After

the partial trace $\mathrm{Tr_B}$ over the bath degrees of freedom, the reduced density matrix (RDM) of the spin system is given by $\rho_{\mathrm{S}}(t) = \mathrm{Tr_B}\{\rho_{\mathrm{tot}}(t)\}$. The time integration of Eq. (17) leads to a formal solution of the RDM,

$$\rho^I_{\mathrm{S}}(t) \ = \mathrm{Tr_B}\left\{\sum_{n=0}^{\infty} \tfrac{1}{n!}\mathcal{T}_+ \left\{\left[-i\int_0^t d\tau \mathcal{L}_{\mathrm{SB}}(\tau)\right]^n \rho_{\mathrm{B}}^{\mathrm{eq}}\right\}\right\} \rho_{\mathrm{S}}(0), \tag{18}$$

where $\mathcal{T}_+$ is the forward time-ordering operator. In Eq. (18), we assume a system-bath factorized initial state with $\rho_{\mathrm{tot}}(0) = \rho_{\mathrm{S}} \otimes \rho_{\mathrm{B}}^{\mathrm{eq}}$, where $\rho_{\mathrm{B}}^{\mathrm{eq}} \propto \exp(-\beta H_{\mathrm{B}})$ is the equilibrium distribution of an isolated bath.

Furthermore, $\rho^I_{\mathrm{S}}(t)$ can be written in the cumulant expansion form

$$\rho^I_{\mathrm{S}}(t) \ = \sum_{n=0}^{\infty} \rho^I_{\mathrm{S},n}(t), \tag{19}$$

and each term is

$$\rho^I_{\mathrm{S},n}(t) \ = \mathrm{Tr_B}\left\{\tfrac{1}{n!}\mathcal{T}_+ \left\{\left[-i\int_0^t d\tau \mathcal{L}_{\mathrm{SB}}(\tau)\right]^n \rho_{\mathrm{B}}^{\mathrm{eq}}\right\}\right\} \rho_{\mathrm{S}}(0). \tag{20}$$

To simplify the cumulant expansion of Eq. (19), all odd terms vanish due to the Gaussian property of the bosonic bath, $\rho^I_{\mathrm{S},2m+1}(t) = 0$. As for the left even terms, after applying the Wick theorem, all the bosonic position operator in $H_{\mathrm{SB}}$ can be arranged together in time order. Hence all the left even terms can be further combined as

$$\rho^I_{\mathrm{S},2m}(t) \ = \tfrac{1}{m!}\mathcal{T}_+ \left\{\left[-\int_0^t d\tau \mathcal{W}(\tau)\right]^m\right\} \rho_{\mathrm{S}}(0). \tag{21}$$

here the transition rate kernel $\mathcal{W}(t)$ is given by

$$\mathcal{W}(t) = \int_0^t d\tau \mathcal{L}_z(t) C_R(t-\tau)\mathcal{L}_z(\tau) + i\mathcal{L}_z(t) C_{\mathrm{I}}(t-\tau)\mathcal{S}_z(\tau). \tag{22}$$

Finally, the reduced density matrix can be simplified into

$$\begin{aligned}\rho^I_{\mathrm{S}}(t) \ &= \sum_{m=0}^{\infty} \frac{1}{m!}\mathcal{T}_+ \left\{\left[-\int_0^t d\tau \mathcal{W}(\tau)\right]^m\right\} \rho_{\mathrm{S}}(0), \\ &= \mathcal{U}_{\mathrm{RDM}}(t)\rho_{\mathrm{S}}(0),\end{aligned} \tag{23}$$

where the time propagator of the RDM is written in a time-ordered exponential form,

$$\mathcal{U}_{\mathrm{RDM}}(t) = \sum_{m=0}^{\infty} \frac{1}{m!}\mathcal{T}_+ \left\{\left[-\int_0^t d\tau \mathcal{W}(\tau)\right]^m\right\}. \tag{24}$$

The bath time correlation function $C(t)$ plays a key role in the extended HEOM. It appears in the transition rate kernel $\mathcal{W}(t)$ and can depict the influence of bosonic bath exert to the reduced dynamics. In the extended HEOM, the bath time correlation function can be expanded using the complete basis function in principle,

$$C(t) = \sum_n a_{\mathrm{R};n}\varphi_{\mathrm{R};n}(t) + i\sum_m a_{\mathrm{I};m}\varphi_{\mathrm{I};m}(t), \tag{25}$$

where $\{\varphi_{\mathrm{R};n}(t), a_{\mathrm{R};n}\}$ and $\{\varphi_{\mathrm{I};m}(t), a_{\mathrm{I};m}\}$ are two sets of basis functions and their coefficients. The time derivative of the basis function is closed, i.e.,

$$d_t\varphi_{\mathrm{X};n}(t) = \sum_{n'} \eta_{\mathrm{X};n,n'}\varphi_{\mathrm{X};n'}(t). \tag{26}$$

The coefficients $\{\eta_{\mathrm{X};n,n'}\}$ leads to a matrix representation of the operator $d_t$ with respect to the set $\{\varphi_{\mathrm{X};n}(t)\}$.

By doing the time derivation of the reduced density matrix, a series of auxiliary density operators are obtained. All the necessary influence that the bath exerts to the system's reduced dynamics is carried by the auxiliary fields $\sigma_{h\geq 1}(t)$. Specifically, for a system-bath factorized initial state, a general $h$-th order ADO is written as

$$\begin{aligned}\sigma_h^{\binom{n_1,\cdots,n_k}{m_1,\cdots,m_l}}(t) &= \mathcal{U}_{\mathrm{S}}(t)\mathcal{T}_+\Big\{\int_0^t d\tau_1\varphi_{\mathrm{R};n_1}(t-\tau_1)[-i\mathcal{L}_z(\tau_1)] \\ &\quad\times\cdots\int_0^t d\tau_k\varphi_{\mathrm{R};n_k}(t-\tau_k)[-i\mathcal{L}_z(\tau_k)]\times\int_0^t d\tau_1'\varphi_{\mathrm{I};m_1}(t-\tau_1')\mathcal{S}_z(\tau_1') \\ &\quad\times\cdots\int_0^t d\tau_l'\varphi_{\mathrm{I};m_l}(t-\tau_l')\mathcal{S}_z(\tau_l')\mathcal{U}_{\mathrm{RDM}}(t)\Big\}\rho_{\mathrm{S}}(0). \end{aligned} \tag{27}$$

In Eq. (27), $\mathcal{U}_{\mathrm{S}}=\exp{(-i\mathcal{L}_{\mathrm{S}}t)}$ is the time propagator of the system and $\mathcal{L}_{\mathrm{S}}=[H_{\mathrm{S}},\dots]$ is the commutator of the system Hamiltonian. The commutator $\mathcal{L}_z=[\sigma_z,\cdots]$ and anti-commutator $\mathcal{S}_z=[\sigma_z,\cdots]_+$ are incorporated of the Pauli-$z$ matrix. As for the formal time propagator of the RDM, it is denoted as $\mathcal{U}_{\mathrm{RDM}}(t)=\mathcal{T}_+\exp{[-\int_0^\infty\mathcal{W}(\tau)\,d\tau]}$ in the interaction picture, where the transition rate kernel reads

$$\mathcal{W}(\tau)=\int_0^\tau d\tau\,[\mathcal{L}_z(t)C_{\mathrm{R}}(t-\tau)\mathcal{L}_z(\tau)+i\mathcal{L}_z(t)C_{\mathrm{I}}(t-\tau)\mathcal{S}_z(\tau)]\,. \tag{28}$$

The hierarchical expansion order is given by the total number of basis functions, i.e., $h=k+l$. Specially, the single zeroth order ($h=0$) ADO is the system's reduced density matrix exactly, i.e., $\sigma_0(t)=\rho_{\mathrm{S}}(t)$. Here the $h$-th order ADO defined in Eq. (27) is characterized by its two sequences, $\{n_1,\cdots,n_k\}$ and $\{m_1,\cdots,m_l\}$, which refer to the basis functions of the bath correlation function,

$$\begin{pmatrix} n_1, & \cdots & ,n_k \\ m_1, & \cdots & ,m_l\end{pmatrix}\Leftrightarrow\left\{\begin{array}{ccc}\varphi_{\mathrm{R};n_1}(\tau_1), & \cdots & ,\varphi_{\mathrm{R};n_k}(\tau_k) \\ \varphi_{\mathrm{I};m_1}(\tau_1'), & \cdots & ,\varphi_{\mathrm{I};m_l}(\tau_l')\end{array}\right\}. \tag{29}$$

All the auxiliary density operators can form a complete dynamic set $\boldsymbol{\sigma}(t)=\{\sigma_0(t)=\rho_{\mathrm{S}}(t),\sigma_1(t),\sigma_2(t),\cdots\}$.

The time evolution of the ADOs is determined by its time derivation. The time derivation of a general $h$-th order ADO includes four different types: (i) The time derivative of the system time propagator $\mathcal{U}_{\mathrm{S}}(t)=\exp(-i\mathcal{L}_{\mathrm{S}}t)$ leads to the system Liouville superoperator,

$$\partial_t\mathcal{U}_{\mathrm{S}}(t)=-i\mathcal{L}_{\mathrm{S}}\exp(-i\mathcal{L}_{\mathrm{S}}t)=-i\mathcal{L}_{\mathrm{S}}\mathcal{U}_{\mathrm{S}}(t). \tag{30}$$

(ii) The derivative of the time integration is formulated as

$$\begin{aligned}\partial_t\mathcal{T}_+\Big\{\cdots\int_0^t d\tau_j\cdots\Big\} &\to \varphi_{X;nj}(0)\mathcal{U}_{\mathrm{S}}(t)[-i\mathcal{O}_X(t)]\mathcal{T}_+\Big\{\cdots\int_0^t d\tau_{j-1}\int_0^t d\tau_{j+1}\cdots\Big\} \\ &= \varphi_{X;n_j}(0)\,[-i\mathcal{O}_X]\,\mathcal{U}_{\mathrm{S}}(t)\mathcal{T}_+\Big\{\cdots\int_0^t d\tau_{j-1}\int_0^t d\tau_{j+1}\cdots\Big\},\end{aligned} \tag{31}$$

with $X=\mathrm{R},\mathrm{I}$. The superoperator $\mathcal{O}_X$ denotes $\mathcal{L}_z(X=R)$ and $i\mathcal{S}_z(X=I)$ accordingly.

(iii) The derivative of the basis set function,

$$\partial_t\mathcal{T}_+\{\cdots\varphi_{X;n_j}(t-\tau_1)\cdots\}=\sum_{j'=1}^{N_X}\eta_{X;j,j'}\mathcal{T}_+\{\cdots\varphi_{X;n_j'}(t-\tau_1)\cdots\}, \tag{32}$$

which is based on the time derivative, $d_t\phi_{X;j}(t) = \sum_{j'} \eta_{X;j,j'}\phi(t)$, due to the completeness of $\{\phi_{X;j}(t)\}$.

(iv) The derivative of the time-ordered integral $\mathcal{U}_{\rm RDM}(t)$ can be organized into

$$\begin{aligned}\partial_t\mathcal{T}_+\{\cdots\mathcal{U}_{\rm RDM}(t)\} &= -i\mathcal{L}_z\sum_{n_{k+1}=1}^{N_{\rm R}} a_{{\rm R};N_{k+1}}\mathcal{T}_+\left\{\cdots\int_0^t d\tau_{k+1}\varphi_{{\rm R};n_{k+1}}(t-\tau_{k+1})[-i\mathcal{L}_z(\tau_{k+1})\mathcal{U}_{\rm RDM}(t)]\right\}\\ &\quad -i\mathcal{L}_z\sum_{m_{l+1}=1}^{N_{\rm I}} a_{{\rm I};m_{l+1}}\mathcal{T}_+\left\{\cdots\int_0^t d\tau'_{l+1}\varphi_{{\rm I};m_{l+1}}(t-\tau'_{l+1})[\mathcal{S}_z(\tau'_{l+1})\mathcal{U}_{\rm RDM}(t)]\right. \qquad (33)\end{aligned}$$

After collecting all the above time derivative terms, we finally obtain an extended HEOM [1–3] organized as,

$$\partial_t\boldsymbol{\sigma}(t) = -\boldsymbol{\mathcal{W}}\boldsymbol{\sigma}(t). \qquad (34)$$

where $\boldsymbol{\mathcal{W}}$ is the transition rate matrix and it is a block tri-diagonal rate matrix $\boldsymbol{\mathcal{W}}_{h,h'} = \boldsymbol{\mathcal{W}}_{h,h}\delta_{h',h} + \boldsymbol{\mathcal{W}}_{h,h\pm1}\delta_{h',h\pm1}$.

## III. COMPLEX INITIAL STATES BASED ON SYSTEM-BATH FACTORIZED STATE

Although our above derivation of extended HEOM is based on the assumption of the system-bath factorized state, the (extended) HEOM can be applied to other complex initial conditions in principle. The HEOM is applied to a general Hamiltonian form $H(t) = H_{\rm S}(t) + H_{\rm B} + \xi(t)H_{\rm SB}$. Comparing to original total Hamiltonian in Eq. 1, here the system Hamiltonian $H_{\rm S}$ and the system-bath coupling strength is changeable. Because the crucial part in above derivation is to define the auxiliary field operator by utilizing the decomposition of the bath time correlation function. So if we can keep the bath Hamiltonian $H_{\rm B}$ and the bilinear system-bath coupling form unchanged, the bath correlation function $C(t)$ and the hierarchical structure of the (extended) HEOM will be conserved.

Although our above derivation of extended HEOM is based on the assumption of the system-bath factorized state, the (extended) HEOM can be applied to other complex initial conditions in principle. Because the crucial part in above derivation is to define the auxiliary field operator by utilizing the decomposition of the bath time correlation function. So if we are able to keep the form of $C(t)$, we will also be able to maintain the hierarchical structure of extended HEOM. Specifically, from the system-bath factorized state, we can obtain more complex correlated initial state by varying the Hamiltonian of spin system $H_{\rm S}$ or the coupling strength value between system and bath, i.e. the Kondo parameter $\alpha$ or the renormalized energy $\lambda$. As a demonstration, we will present two typical initial states that can be obtained from the system-bath factorized state $\rho_{\rm fac}(0) = |+\rangle\langle+| \otimes \rho_{\rm B}^{\rm eq}$, i.e., local equilibrium initial state and the excited equilibrium initial state.

### A. Local Equilibrium Initial State

Local equilibrium state is the state that each site reach a local thermal equilibrium with its local environment. Every site is prepared to be decoupled with each other initially. Be different with the system-bath factorized state, the system and bath is correlated in the local equilibrium state.

$\rho_{\rm fac}(0) \to H_{\rm S}(\Delta\sigma_x = 0) \to \rho_{\rm loc}^{\rm eq} \to H_{\rm S}(\Delta\sigma_x \neq 0)$ As a demonstration, for the SBM, we show how to obtain the local equilibrium state from the system-bath factorized initial state by varying the system's Hamiltonian. (1) Initially, we start from the system-bath factorized initial state $\rho_{\rm fac}(0) = |+\rangle\langle+| \otimes \rho_{\rm B}^{\rm eq}$. (2) Then each site is prepared to be independent with each other, which means the coupling terming $\Delta\sigma_x = 0$ should be vanish in the system Hamiltonian $H_{\rm S} = \Delta\sigma_x$. (3) After a long evolution, each site reach the local equilibrium with its surrounded environment. (4) Subsequently, we obtain the local equilibrium initial state as $\rho_{\rm tot}(0) = |+\rangle\langle+| \otimes \rho_+^{\rm eq}$ with $\rho_+^{\rm eq} \propto \exp[-\beta(\sigma_z \sum_j c_j q_j + H_{\rm B})]$. Finally, we need to recover the coupling term $\Delta\sigma_x$ in $H_{\rm S}$ and set the system in the spin up state $\rho_{\rm S}(0) = |+\rangle\langle+|$. The whole procedure can be summarized as

$$\rho_{\rm fac}(0) \xrightarrow{H_{\rm S}(\Delta=0)} \rho_{\rm loc}^{\rm eq} \xrightarrow{H_{\rm S}(\Delta\neq0)}$$

For the local equilibrium initial state, the zeroth order ADO $\boldsymbol{\sigma}_0(t) = \rho_{\rm S}(t)$ is still the reduced density matrix in physics, and it still obey the extended HEOM.

### B. Initial State in Our Calculation

In this paper, the initial condition applied to calculate the linear response function can also be constructed from the system-bath factorized initial state. Firstly, starting from the system-bath factorized state, we use the extended HEOM to propagate the total system to reach its equilibrium state $\boldsymbol{\sigma}^{\rm eq}$. Then the total initial perturbed elements is excited by the external interaction at $t = 0$. Thus the new initial state in our calculation is obtained as $\tilde{\boldsymbol{\sigma}}(0) = \mathcal{L}_z\boldsymbol{\sigma}^{\rm eq}$. Noticing that, for the new initial state, the current zeroth order ADO $\tilde{\boldsymbol{\sigma}}_0(0) = \mathcal{L}_z\boldsymbol{\sigma}_0^{\rm eq}$ is not the usual RDM. The whole procedure can be summarized as

$$\rho_{\rm fac}(0) \longrightarrow \rho_{\rm tot}^{\rm eq} \Leftrightarrow \boldsymbol{\sigma}^{\rm eq} \longrightarrow \tilde{\boldsymbol{\sigma}}(0) = \mathcal{L}_z\boldsymbol{\sigma}^{\rm eq}$$

Now that we have obtained a new initial state, we have to ask whether it still follows the extended HEOM. Surely, since the form of the bath time correlation function has not changed, the hierarchical structure of the extended HEOM can be retained. In HEOM, all the ADOs can form the complete dynamic set $\boldsymbol{\sigma}(t)$. Based on the complete dynamic set $\boldsymbol{\sigma}(t)$, a great resemblance between quantum operators and HEOM matrices can be observed. In Ref. [4], Z. H. Gong *et al.* found, due to the ADOs set $\boldsymbol{\sigma}(t)$ is a dynamic complete set of reduced quantum dissipation, there is an one-to-one mapping between quantum operators and HEOM matrices. Specifically, considering the trace over bath degrees of freedom ${\rm Tr}_{\rm B}\{\cdots\}$, the mapping applied for Eq.(14) is

$$\begin{cases} {\rm Tr}_{\rm B}\{\cdots\rho_{\rm tot}\} & \Leftrightarrow & {\rm Tr}_{\rm B}\{\cdots\boldsymbol{\sigma}(t)\}, \\ {\rm Tr}_{\rm B}\{e^{-i\mathcal{L}t}\cdots\} & \Leftrightarrow & {\rm Tr}_{\rm B}\{e^{-\boldsymbol{\mathcal{W}}t}\cdots\}. \end{cases} \tag{35}$$

Thus Eq. (10) can be re-expressed as

$$\begin{aligned} \chi(t) &= i\Theta(t){\rm Tr}_{\rm S}\{\sigma_z{\rm Tr}_{\rm B}\{e^{-i\mathcal{L}t}(\mathcal{L}_z\rho_{\rm tot}^{\rm eq})\}\}\mu_z^2, \\ &= i\Theta(t){\rm Tr}_{\rm S}\{\sigma_z{\rm Tr}_{\rm B}\{e^{-\boldsymbol{\mathcal{W}}t}(\mathcal{L}_z\boldsymbol{\sigma}^{\rm eq})\}\}\mu_z^2, \\ &= i\Theta(t){\rm Tr}_{\rm S}\{\sigma_z{\rm Tr}_{\rm B}\{e^{-\boldsymbol{\mathcal{W}}t}\tilde{\boldsymbol{\sigma}}(0)\}\}\mu_z^2, \end{aligned} \tag{36}$$

where $\boldsymbol{\sigma}^{\rm eq}$ is the stationary ADO vector in the equilibrium state. The perturbed elements is the ADOs in equilibrium excited by the external interaction, which is noted as $\tilde{\boldsymbol{\sigma}}(0) = \mathcal{L}_z \boldsymbol{\sigma}^{\rm eq}$. In the HEOM's formalism, considering the partial trace $\mathrm{Tr_B}\{\cdots\}$ over bath freedom, the total density matrix $\rho_{\rm tot}(t)$ and the total Liouville superoperator $i\mathcal{L}_{\rm tot}$ are transformed into the complete dynamic basis set $\boldsymbol{\sigma}(t)$ and the transition rate matrix $\boldsymbol{\mathcal{W}}$. $\mathrm{Tr_B}\{\cdots \rho_{\rm tot}\}$ is mapped to $\mathrm{Tr_B}\{\cdots \boldsymbol{\sigma}\}$. Noted that the operator $\mathcal{L}_z$ in $\tilde{\boldsymbol{\sigma}}$ does not dependent on the bath. So this term $\mathrm{Tr_B}\{e^{-i\mathcal{L}t}(\mathcal{L}_z \rho^{\rm eq}_{\rm tot})\}$ can be expressed as $\mathrm{Tr_B}\{e^{-\boldsymbol{\mathcal{W}}t}(\mathcal{L}_z \boldsymbol{\sigma}^{\rm eq})\}$. More detailed derivation can see Ref. [5].

When the external interaction is exerted to the spin system, the bath environment keeps invariant, so the HEOM's transition rate matrix $\boldsymbol{\mathcal{W}}$ will remain the same with the initial time. Furthermore, according to the mapping rule from quantum operator to HEOM's matrix, the time evolution propagator is replaced by the HEOM transition rate matrix $\boldsymbol{\mathcal{W}}$. Thus the propagation of the perturbed elements $\tilde{\boldsymbol{\sigma}}(t)$ also obey the extended HEOM,

$$\partial_t \tilde{\boldsymbol{\sigma}}(t) \; = -\boldsymbol{\mathcal{W}} \tilde{\boldsymbol{\sigma}}(t), \tag{37}$$

here the initial value of $\tilde{\boldsymbol{\sigma}}(t)$ is $\tilde{\boldsymbol{\sigma}}(0) = \mathcal{L}_z \boldsymbol{\sigma}^{\rm eq}$. Thus the procedure to calculate the linear response function with extended HEOM is straightforward. Firstly, from Eq.(13), in order to calculate the linear response function with kinetic method, it is required to propagate the SBM to its equilibrium state. At $t=0$, the system in equilibrium is excited by the external interaction, which corresponds to $\tilde{\boldsymbol{\sigma}}(0) = \mathcal{L}_z \boldsymbol{\sigma}^{\rm eq}$. The extended HEOM is used to propagate $\tilde{\boldsymbol{\sigma}}(0)$ from the new initial state. Then we take the trace over the system's degrees of freedom. Finally, the linear absorption spectra $\mathrm{Im}\,\chi(\omega)$ can be obtained from the imaginary part of its Fourier transformation,

$$\chi''(\omega) = \mathrm{Im} \int_{-\infty}^{\infty} \chi(t) e^{i\omega t}\, dt. \tag{38}$$


[1] Z. F. Tang, X. L. Ouyang, Z. H. Gong, H. B. Wang, and J. L. Wu, J. Chem. Phys. **143**, 224112 (2015).

[2] C. R. Duan, Z. F. Tang, J. S. Cao, and J. L. Wu, Phys. Rev. B **95**, 214308 (2017).

[3] C. R. Duan, Q. L. Wang, Z. F. Tang, and J. L. Wu, J. Chem. Phys. **147**, 164112 (2017).

[4] Z. H. Gong, Z. F. Tang, H. B. Wang and J. L. Wu, J. Chem. Phys. **147**, 244112 (2017)

[5] S. K. Wang, X. Zheng, J. S. Jin and Y. J. Yan, Phys. Rev. B **88**, 035129 (2013)
